# Supplementary material for: Pseudopotentials for high-throughput DFT calculations
Source: arXiv:1305.5973 source file (2013-08-16)
Supplement: Supplementary file 1 [file psp_supp.pdf]

# Pseudopotentials for high-throughput DFT calculations: supplementary material

Kevin F. Garrity, Joseph W. Bennett, Karin M. Rabe, and David Vanderbilt
*Department of Physics & Astronomy, Rutgers University,*
*Piscataway, New Jersey 08854-8019, USA*

(Dated: August 15, 2013)

Supplementary material for "Pseudopotentials for high-throughput DFT calculations". Note that these results are intended for pseudopotential testing and should be compared only to other calculations with identical approximations and convergence parameters (see text). They are not intended to correspond to experiment.

TABLE I: Testing data for lattice constants (Å) of *fcc* and *bcc* lattices. Entries marked with – were unable to be converged to sufficient accuracy for comparison.

| Element | $a_{\mathrm{AE}}$ *fcc* | $a_{\mathrm{GBRV}}$ *fcc* | $a_{\mathrm{VASP}}$ *fcc* | $a_{\mathrm{PSLIB}}$ *fcc* | $a_{\mathrm{AE}}$ *bcc* | $a_{\mathrm{GBRV}}$ *bcc* | $a_{\mathrm{VASP}}$ *bcc* | $a_{\mathrm{PSLIB}}$ *bcc* |
|---|---|---|---|---|---|---|---|---|
| H | 2.283 | 2.284 | 2.283 | 2.284 | 1.806 | 1.807 | 1.807 | 1.806 |
| Li | 4.335 | 4.332 | 4.336 | 4.359 | 3.427 | 3.425 | 3.429 | 3.454 |
| Be | 3.166 | 3.175 | 3.170 | 3.160 | 2.506 | 2.514 | 2.508 | 2.501 |
| B | 2.872 | 2.873 | 2.872 | 2.871 | 2.323 | 2.325 | 2.323 | 2.322 |
| C | 3.103 | 3.103 | 3.104 | 3.103 | 2.366 | 2.366 | 2.367 | 2.365 |
| O | 3.178 | 3.175 | 3.172 | 3.172 | 2.511 | 2.511 | 2.508 | 2.508 |
| N | – | 3.123 | 3.117 | 3.117 | – | 2.456 | 2.449 | 2.449 |
| F | 3.447 | 3.430 | 3.433 | 3.433 | 2.730 | 2.714 | 2.717 | 2.720 |
| Na | 5.294 | 5.294 | 5.292 | 5.294 | 4.199 | 4.196 | 4.205 | 4.195 |
| Mg | 4.526 | 4.527 | 4.530 | 4.521 | 3.581 | 3.582 | 3.582 | 3.577 |
| Al | 4.043 | 4.043 | 4.044 | 4.040 | 3.242 | 3.242 | 3.242 | 3.239 |
| Si | 3.857 | 3.853 | 3.859 | 3.852 | 3.080 | 3.076 | 3.078 | 3.075 |
| P | – | 3.917 | 3.893 | 3.889 | – | 3.060 | 3.043 | 3.041 |
| S | 3.994 | 3.992 | 3.993 | 3.988 | 3.182 | 3.178 | 3.180 | 3.175 |
| Cl | 4.409 | 4.396 | 4.395 | 4.392 | 3.501 | 3.491 | 3.492 | 3.488 |
| K | 6.684 | 6.668 | 6.670 | 6.667 | 5.294 | 5.279 | 5.285 | 5.281 |
| Ca | 5.532 | 5.523 | 5.529 | 5.514 | 4.400 | 4.392 | 4.396 | 4.386 |
| Sc | 4.622 | 4.621 | 4.624 | 4.623 | 3.680 | 3.679 | 3.683 | 3.681 |
| Ti | 4.114 | 4.114 | 4.110 | 4.105 | 3.259 | 3.258 | 3.255 | 3.249 |
| V | 3.822 | 3.820 | 3.823 | 3.824 | 3.006 | 3.003 | 3.005 | 3.006 |
| Cr | 3.630 | 3.629 | 3.625 | 3.634 | 2.851 | 2.849 | 2.848 | 2.861 |
| Mn | 3.503 | 3.502 | 3.501 | 3.508 | 2.784 | 2.784 | 2.783 | 2.788 |
| Fe | 3.449 | 3.451 | 3.447 | 3.457 | 2.762 | 2.762 | 2.758 | 2.770 |
| Co | 3.457 | 3.455 | 3.457 | 3.463 | 2.762 | 2.761 | 2.761 | 2.766 |
| Ni | 3.515 | 3.511 | 3.516 | 3.517 | 2.793 | 2.790 | 2.794 | 2.795 |
| Cu | 3.638 | 3.639 | 3.641 | 3.654 | 2.885 | 2.886 | 2.885 | 2.896 |
| Zn | 3.936 | 3.936 | 3.939 | 3.931 | 3.128 | 3.128 | 3.130 | 3.127 |
| Ga | 4.240 | 4.244 | 4.242 | 4.247 | 3.364 | 3.366 | 3.364 | 3.369 |
| Ge | 4.283 | 4.282 | 4.283 | 4.283 | 3.397 | 3.396 | 3.397 | 3.396 |
| As | 4.272 | 4.276 | 4.273 | 4.272 | 3.383 | 3.386 | 3.385 | 3.383 |
| Se | 4.337 | 4.332 | 4.335 | 4.341 | 3.460 | 3.456 | 3.459 | 3.463 |
| Br | 4.732 | 4.726 | 4.726 | 4.731 | 3.765 | 3.762 | 3.762 | 3.765 |
| Rb | 7.183 | 7.155 | 7.160 | 7.155 | 5.680 | 5.659 | 5.665 | 5.659 |
| Sr | 6.030 | 6.022 | 6.022 | 6.020 | 4.756 | 4.750 | 4.749 | 4.748 |
| Y | 5.062 | 5.057 | 5.055 | 5.060 | 4.044 | 4.040 | 4.040 | 4.042 |
| Zr | 4.522 | 4.520 | 4.521 | 4.527 | 3.569 | 3.566 | 3.568 | 3.572 |
| Nb | 4.217 | 4.214 | 4.215 | 4.217 | 3.309 | 3.306 | 3.307 | 3.308 |
| Mo | 4.007 | 4.002 | 4.008 | 4.005 | 3.166 | 3.160 | 3.164 | 3.162 |
| Tc | 3.875 | 3.872 | 3.876 | 3.874 | 3.082 | 3.080 | 3.085 | 3.082 |
| Ru | 3.809 | 3.806 | 3.808 | 3.809 | 3.058 | 3.054 | 3.056 | 3.057 |
| Rh | 3.836 | 3.836 | 3.834 | 3.842 | 3.071 | 3.069 | 3.069 | 3.075 |
| Pd | 3.951 | 3.951 | 3.951 | 3.956 | 3.137 | 3.136 | 3.135 | 3.141 |
| Ag | 4.158 | 4.161 | 4.165 | 4.167 | 3.299 | 3.299 | 3.303 | 3.304 |
| Cd | 4.511 | 4.512 | 4.515 | 4.491 | 3.628 | 3.629 | 3.632 | 3.612 |
| In | 4.795 | 4.800 | 4.797 | 4.793 | 3.827 | 3.831 | 3.826 | 3.825 |
| Sn | 4.824 | 4.826 | 4.824 | 4.830 | 3.823 | 3.825 | 3.823 | 3.829 |
| Sb | 4.805 | 4.808 | 4.802 | 4.782 | 3.807 | 3.809 | 3.805 | 3.787 |
| Te | 4.840 | 4.840 | 4.837 | 4.854 | 3.867 | 3.865 | 3.865 | 3.877 |
| I | 5.201 | 5.195 | 5.198 | 5.192 | 4.149 | 4.149 | 4.151 | 4.144 |
| Cs | 7.821 | 7.789 | 7.794 | 7.808 | 6.172 | 6.147 | 6.145 | 6.161 |
| Ba | 6.347 | 6.338 | 6.345 | 6.344 | 5.023 | 5.018 | 5.023 | 5.023 |
| La | 5.267 | 5.277 | 5.290 | 5.387 | 4.235 | 4.239 | 4.248 | 4.297 |
| Hf | 4.488 | 4.491 | 4.483 | 4.483 | 3.551 | 3.554 | 3.549 | 3.548 |
| Ta | 4.235 | 4.232 | 4.235 | 4.227 | 3.333 | 3.331 | 3.332 | 3.327 |
| W | 4.041 | 4.042 | 4.042 | 4.046 | 3.188 | 3.187 | 3.187 | 3.190 |
| Re | 3.917 | 3.915 | 3.919 | 3.919 | 3.118 | 3.115 | 3.120 | 3.119 |
| Os | 3.858 | 3.855 | 3.861 | 3.861 | 3.096 | 3.091 | 3.099 | 3.103 |
| Ir | 3.881 | 3.875 | 3.877 | 3.888 | 3.113 | 3.107 | 3.110 | 3.118 |
| Pt | 3.970 | 3.964 | 3.970 | 3.984 | 3.166 | 3.160 | 3.165 | 3.176 |
| Au | 4.168 | 4.163 | 4.166 | 4.180 | 3.306 | 3.302 | 3.304 | 3.316 |
| Hg | – | - | – | – | – | - | – | – |
| Tl | 4.996 | 5.004 | 4.997 | 4.962 | 3.977 | 3.980 | 3.975 | 3.974 |
| Pb | 5.045 | 5.039 | 5.044 | 5.044 | 4.008 | 4.003 | 4.007 | 4.007 |
| Bi | 5.038 | 5.035 | 5.035 | 5.041 | 3.984 | 3.981 | 3.982 | 3.979 |

TABLE II: Testing data for lattice constants (Å) of rock salt structures. Entries marked with − were unable to be converged to sufficient accuracy for comparison.

| Element | $a_{\mathrm{AE}}$ | $a_{\mathrm{GBRV}}$ | $a_{\mathrm{VASP}}$ | $a_{\mathrm{PSLIB}}$ |
|---|---|---|---|---|
| LiCl | 5.161 | 5.151 | 5.150 | 5.160 |
| NaCl | 5.714 | 5.701 | 5.701 | 5.696 |
| KCl | 6.391 | 6.382 | 6.391 | 6.384 |
| RbCl | 6.710 | 6.698 | 6.705 | 6.701 |
| CsCl | 7.088 | 7.072 | 7.085 | 7.088 |
| BeO | 3.650 | 3.653 | 3.654 | 3.638 |
| MgO | 4.259 | 4.259 | 4.261 | 4.250 |
| CaO | 4.839 | 4.834 | 4.842 | 4.828 |
| SrO | 5.204 | 5.198 | 5.208 | 5.201 |
| BaO | 5.590 | 5.597 | 5.617 | 5.603 |
| ScN | 4.516 | 4.514 | 4.519 | 4.516 |
| YN | 4.911 | 4.908 | 4.906 | 4.915 |
| LaN | 5.314 | 5.314 | 5.328 | 5.349 |
| TiO | 4.288 | 4.288 | 4.288 | 4.283 |
| VO | 4.192 | 4.190 | 4.191 | 4.192 |
| CrO | 4.139 | 4.139 | 4.134 | 4.142 |
| MnO | 4.108 | 4.110 | 4.103 | 4.110 |
| FeO | 4.096 | 4.103 | 4.092 | 4.103 |
| CoO | 4.106 | 4.108 | 4.102 | 4.108 |
| NiO | 4.166 | 4.170 | 4.167 | 4.169 |
| CuO | 4.248 | 4.250 | 4.246 | 4.260 |
| ZnO | 4.332 | 4.338 | 4.340 | 4.330 |
| ZrO | 4.608 | 4.605 | 4.607 | 4.621 |
| NbO | 4.476 | 4.474 | 4.471 | 4.475 |
| MoO | 4.419 | 4.417 | 4.419 | 4.417 |
| TcO | 4.398 | 4.396 | 4.394 | 4.394 |
| RuO | 4.411 | 4.408 | 4.405 | 4.408 |
| RhO | 4.450 | 4.455 | 4.449 | 4.455 |
| PdO | 4.544 | 4.550 | 4.541 | 4.547 |
| AgO | 4.677 | 4.680 | 4.675 | 4.684 |
| CdO | 4.774 | 4.783 | 4.785 | 4.762 |
| HfO | 4.611 | 4.596 | 4.584 | 4.574 |
| TaO | 4.506 | 4.503 | 4.504 | 4.483 |
| WO | 4.466 | 4.470 | 4.467 | 4.466 |
| ReO | 4.455 | 4.459 | − | 4.461 |
| OsO | 4.487 | 4.487 | 4.497 | 4.492 |
| IrO | 4.542 | 4.540 | 4.545 | 4.548 |
| PtO | 4.624 | 4.621 | 4.622 | 4.637 |
| AuO | 4.759 | 4.754 | 4.752 | 4.769 |
| HgO | 4.929 | 4.933 | 4.938 | 4.913 |
| BN | 3.506 | 3.506 | 3.505 | 3.504 |
| AlN | 4.073 | 4.079 | 4.070 | 4.068 |
| GaN | 4.269 | 4.275 | 4.274 | 4.285 |
| InN | 4.708 | 4.713 | 4.711 | 4.714 |
| TlN | 4.957 | 4.963 | 4.963 | 4.968 |
| CO | 3.977 | 3.982 | 3.974 | 3.972 |
| SiO | 4.616 | 4.617 | 4.615 | 4.612 |
| GeO | 4.773 | 4.775 | 4.773 | 4.772 |
| SnO | 5.120 | 5.122 | 5.119 | 5.125 |
| PbO | 5.269 | 5.263 | 5.266 | 5.268 |
| AlN | 4.073 | 4.079 | 4.070 | 4.068 |
| AlP | 5.075 | 5.077 | 5.072 | 5.068 |
| AlAs | 5.303 | 5.307 | 5.298 | 5.301 |
| AlSb | 5.774 | 5.761 | 5.765 | 5.752 |
| AlBi | 5.987 | 5.976 | 5.977 | 5.976 |
| SrS | 6.063 | 6.057 | 6.065 | 6.060 |
| SrSe | 6.301 | 6.297 | 6.304 | 6.300 |
| SrTe | 6.724 | 6.720 | 6.726 | 6.728 |
| LiF | 4.076 | 4.074 | 4.067 | 4.081 |
| LiBr | 5.521 | 5.512 | 5.511 | 5.524 |
| LiI | 6.038 | 6.020 | 6.021 | 6.030 |
| NaF | 4.711 | 4.717 | 4.708 | 4.705 |
| NaBr | 6.049 | 6.040 | 6.040 | 6.037 |
| NaI | 6.540 | 6.534 | 6.537 | 6.529 |

TABLE III: Testing data for lattice constants (Å) of perovskite and anti-perovskite structures. Entries marked with − were unable to be converged to sufficient accuracy for comparison.

| Element | $a_{AE}$ | $a_{GBRV}$ | $a_{VASP}$ | $a_{PSLIB}$ |
|---|---|---|---|---|
| $SrLiF_3$ | 3.884 | 3.881 | 3.884 | 3.884 |
| $NaNbO_3$ | 3.981 | 3.981 | 3.976 | 3.980 |
| $KMgF_3$ | 4.059 | 4.057 | 4.062 | 4.052 |
| $CsMgF_3$ | 4.258 | 4.255 | 4.261 | 4.255 |
| $MgTiO_3$ | 3.839 | 3.840 | 3.839 | 3.839 |
| $CaTiO_3$ | 3.886 | 3.887 | 3.888 | 3.886 |
| $SrTiO_3$ | 3.941 | 3.942 | 3.943 | 3.942 |
| $BaTiO_3$ | 4.024 | 4.031 | 4.035 | 4.030 |
| $BiScO_3$ | 4.074 | 4.074 | 4.079 | 4.076 |
| $BiYO_3$ | 4.335 | 4.334 | 4.331 | 4.343 |
| $SrVO_3$ | 3.862 | 3.863 | 3.866 | 3.867 |
| $SrCrO_3$ | 3.820 | 3.821 | 3.819 | 3.826 |
| $SrMnO_3$ | 3.799 | 3.800 | 3.798 | 3.808 |
| $SrFeO_3$ | 3.801 | 3.802 | 3.802 | 3.812 |
| $SrCoO_3$ | 3.811 | 3.810 | 3.812 | 3.823 |
| $SrNiO_3$ | 3.843 | 3.842 | 3.849 | 3.853 |
| $KNiF_3$ | 4.039 | 4.036 | 4.036 | 4.042 |
| $KCuF_3$ | 4.085 | 4.084 | 4.084 | 4.095 |
| $KZnF_3$ | 4.132 | 4.133 | 4.139 | 4.130 |
| $SrZrO_3$ | 4.176 | 4.175 | 4.177 | 4.187 |
| $SrNbO_3$ | 4.067 | 4.066 | 4.064 | 4.066 |
| $SrMoO_3$ | 4.002 | 4.001 | 4.003 | 4.002 |
| $SrTcO_3$ | 3.967 | 3.968 | 3.966 | 3.968 |
| $SrRuO_3$ | 3.959 | 3.959 | 3.956 | 3.962 |
| $SrRhO_3$ | 3.982 | 3.987 | 3.981 | 3.991 |
| $KPdF_3$ | 4.312 | 4.314 | 4.309 | 4.315 |
| $SrAgF_3$ | 4.536 | 4.535 | 4.535 | 4.537 |
| $KCdF_3$ | 4.463 | 4.471 | 4.477 | 4.458 |
| $LaAlO_3$ | 3.816 | 3.819 | 3.822 | 3.829 |
| $SrHfO_3$ | 4.155 | 4.148 | 4.146 | 4.133 |
| $SrTaO_3$ | 4.066 | 4.067 | 4.067 | 4.050 |
| $SrWO_3$ | 4.014 | 4.020 | 4.019 | 4.013 |
| $SrReO_3$ | 3.986 | 3.989 | 3.997 | 3.994 |
| $SrOsO_3$ | 3.982 | 3.983 | 3.992 | 3.988 |
| $SrIrO_3$ | 3.994 | 3.996 | 4.006 | 4.018 |
| $SrPtO_3$ | 4.040 | 4.039 | 4.039 | 4.079 |
| $BiAuO_3$ | 4.151 | 4.152 | 4.147 | 4.171 |
| $KHgF_3$ | 4.594 | 4.602 | 4.608 | 4.587 |
| $TlCTi_3$ | 4.263 | 4.261 | 4.260 | 4.259 |
| $LaBRh_3$ | 4.288 | 4.283 | 4.287 | 4.306 |
| $BiAlO_3$ | 3.797 | 3.800 | 3.795 | 3.795 |
| $BiInO_3$ | 4.170 | 4.175 | 4.178 | 4.179 |
| $SrSiO_3$ | 3.695 | 3.695 | 3.698 | 3.694 |
| $SrGeO_3$ | 3.855 | 3.860 | 3.860 | 3.865 |
| $SnTiO_3$ | 3.949 | 3.950 | 3.949 | 3.950 |
| $PbTiO_3$ | 3.971 | 3.970 | 3.971 | 3.971 |
| $PNCa_3$ | 4.725 | 4.721 | 4.728 | 4.714 |
| $AsNCa_3$ | 4.769 | 4.766 | 4.772 | 4.759 |
| $SbNCa_3$ | 4.872 | 4.868 | 4.875 | 4.862 |
| $SrTiS_3$ | 4.786 | 4.781 | 4.785 | 4.781 |
| $SrTiSe_3$ | 5.030 | 5.029 | 5.033 | 5.034 |
| $BaZrTe_3$ | 5.681 | 5.679 | 5.684 | 5.691 |
| $KMgCl_3$ | 5.028 | 5.024 | 5.026 | 5.018 |
| $CsPbBr_3$ | 5.994 | 5.999 | 6.003 | 6.009 |
| $CsPbI_3$ | 6.383 | 6.393 | 6.396 | 6.397 |

TABLE IV: Testing data for lattice constants (Å) of half-Heusler structures. Entries marked with − were unable to be converged to sufficient accuracy for comparison. Entries are listed with the inequivalent "stuffing atom" (Wycoff position 4c) third.

| Element | $a_{\mathrm{AE}}$ | $a_{\mathrm{GBRV}}$ | $a_{\mathrm{VASP}}$ | $a_{\mathrm{PSLIB}}$ |
|---|---|---|---|---|
| AgAlGe | 6.224 | 6.220 | 6.223 | 6.221 |
| AgAlSn | 6.595 | 6.594 | 6.596 | 6.600 |
| AgCaBi | 7.161 | 7.155 | 7.163 | 7.153 |
| AgYSi | 6.501 | 6.496 | 6.499 | 6.502 |
| AlBeB | 4.963 | 4.966 | 4.964 | 4.958 |
| AlLiGe | 6.022 | 6.015 | 6.014 | 6.017 |
| AlLiSi | 5.931 | 5.933 | 5.936 | 5.938 |
| AuLiSb | 6.449 | 6.440 | 6.431 | 6.450 |
| BaZnTi | 6.946 | 6.955 | 6.982 | 6.967 |
| BeScB | 5.321 | 5.317 | 5.324 | 5.318 |
| BiMgCu | 6.444 | 6.438 | 6.440 | 6.444 |
| BiScNi | 6.271 | 6.261 | 6.265 | 6.267 |
| BiYNi | 6.502 | 6.494 | 6.495 | 6.501 |
| BiYPd | 6.736 | 6.731 | 6.734 | 6.738 |
| BiZrCo | 6.235 | 6.225 | 6.226 | 6.236 |
| BiZrNi | 6.300 | 6.288 | 6.291 | 6.299 |
| CaZnSn | 6.923 | 6.923 | 6.928 | 6.924 |
| CaZnZr | 6.834 | 6.823 | 6.834 | 6.829 |
| CdPLi | 5.969 | 5.955 | 5.952 | 5.945 |
| CoMnSb | 5.835 | 5.833 | 5.824 | 5.851 |
| CoNbSn | 6.186 | 6.176 | 6.175 | 6.186 |
| CoSnMo | 6.107 | 6.096 | 6.099 | 6.105 |
| CoSnNb | 6.222 | 6.211 | 6.211 | 6.218 |
| CoSnTc | 6.034 | 6.023 | 6.024 | 6.032 |
| CoSnTi | 6.121 | 6.115 | 6.115 | 6.118 |
| CoZrSb | 6.328 | 6.320 | 6.319 | 6.333 |
| CrSbNi | 5.803 | 5.805 | 5.800 | 5.814 |
| CsZnBi | 8.016 | 8.002 | 8.018 | 8.043 |
| CuAlGe | 5.920 | 5.912 | 5.910 | 5.916 |
| CuAlSn | 6.332 | 6.327 | 6.325 | 6.337 |
| CuMgAs | 6.057 | 6.057 | 6.052 | 6.057 |
| CuMgSn | 6.436 | 6.432 | 6.433 | 6.439 |
| CuScSn | 6.461 | 6.456 | 6.459 | 6.467 |
| CuYSi | 6.310 | 6.302 | 6.302 | 6.312 |
| CuYSn | 6.732 | 6.729 | 6.728 | 6.741 |
| FeSnTi | 6.118 | 6.115 | 6.111 | 6.119 |
| InLiGe | 6.398 | 6.397 | 6.394 | 6.397 |
| IrMnSn | 6.044 | 6.033 | 6.032 | 6.050 |
| KZnBi | 7.428 | 7.418 | 7.426 | 7.432 |
| LiAlSn | 6.459 | 6.454 | 6.453 | 6.459 |
| LiAuS | 6.015 | 5.994 | 5.993 | 6.008 |
| LiBaP | 7.139 | 7.148 | 7.164 | 7.158 |
| LiCaP | 6.497 | 6.492 | 6.498 | 6.491 |
| LiCGa | 5.088 | 5.091 | 5.091 | 5.100 |
| LiCuS | 5.578 | 5.576 | 5.574 | 5.594 |
| LiCuSe | 5.863 | 5.859 | 5.858 | 5.880 |
| LiCuTe | 6.273 | 6.273 | 6.261 | 6.294 |
| LiLaGe | 6.930 | 6.927 | 6.934 | 6.960 |
| LiMgN | 5.005 | 5.008 | 5.008 | 5.011 |
| LiSiGa | 5.881 | 5.882 | 5.881 | 5.887 |
| LiSnIn | 6.799 | 6.799 | 6.796 | 6.801 |
| LiSrP | 6.817 | 6.813 | 6.819 | 6.818 |
| LiYSn | 7.009 | 7.006 | 7.005 | 7.014 |
| LiZnN | 4.923 | 4.929 | 4.929 | 4.928 |

TABLE V: Continuation of table IV.

| Element | $a_{AE}$ | $a_{GBRV}$ | $a_{VASP}$ | $a_{PSLIB}$ |
|---|---|---|---|---|
| MgPLi | 5.775 | 5.776 | 5.776 | 5.776 |
| MgSbCu | 6.259 | 6.257 | 6.257 | 6.256 |
| MgSbNi | 6.099 | 6.094 | 6.094 | 6.093 |
| MgSbPd | 6.354 | 6.351 | 6.349 | 6.351 |
| MgSbPt | 6.364 | 6.359 | 6.357 | 6.362 |
| MgSnCu | 6.247 | 6.248 | 6.248 | 6.257 |
| MgSrGe | 7.069 | 7.067 | 7.072 | 7.064 |
| MgSrSi | 7.012 | 7.009 | 7.016 | 7.008 |
| MgSrSn | 7.427 | 7.424 | 7.428 | 7.422 |
| MgZnHf | 6.579 | 6.576 | 6.573 | 6.572 |
| MnPdTe | 6.059 | 6.075 | 6.036 | 6.068 |
| MnPtGa | 5.744 | 5.743 | 5.744 | 5.756 |
| MnPtSb | 6.064 | 6.053 | 6.048 | 6.076 |
| MnRhSb | 6.001 | 5.991 | 5.982 | 6.010 |
| MnSbCo | 5.720 | 5.724 | 5.718 | 5.737 |
| MnSbCu | 5.853 | 5.857 | 5.850 | 5.868 |
| MnSbIr | 6.033 | 6.022 | 6.017 | 6.035 |
| MnSbNi | 5.758 | 5.760 | 5.755 | 5.771 |
| MnSbOs | 6.017 | 6.004 | 6.003 | 6.015 |
| MnSbPt | 6.106 | 6.096 | 6.090 | 6.112 |
| MnSbRe | 6.045 | 6.036 | 6.033 | 6.040 |
| MnSbRh | 5.996 | 5.988 | 5.980 | 5.998 |
| MnSbTa | 6.246 | 6.239 | 6.237 | 6.233 |
| MnSbW | 6.116 | 6.107 | 6.104 | 6.110 |
| MnSnPt | 6.093 | 6.081 | 6.082 | 6.098 |
| NaAgO | 5.708 | 5.711 | 5.709 | 5.706 |
| NaAlGe | 6.387 | 6.384 | 6.386 | 6.380 |
| NaBGe | 5.750 | 5.754 | 5.754 | 5.748 |
| NaMgN | 5.446 | 5.452 | 5.450 | 5.439 |
| NaYGe | 6.897 | 6.897 | 6.899 | 6.899 |
| NaYSn | 7.286 | 7.282 | 7.284 | – |
| NaZnBi | 6.951 | 6.948 | 6.954 | 6.995 |
| NaZnP | 6.150 | 6.148 | 6.149 | 6.143 |
| NaZnSb | 6.765 | 6.765 | 6.764 | 6.764 |
| NbRhSn | 6.295 | 6.289 | 6.289 | 6.301 |
| NbSbFe | 5.972 | 5.963 | 5.956 | 5.970 |
| NbSbRh | 6.220 | 6.215 | 6.213 | 6.220 |
| NbSbRu | 6.197 | 6.191 | 6.189 | – |
| NiHfSn | 6.341 | 6.334 | 6.329 | 6.332 |
| NiSbMn | 5.817 | 5.818 | 5.813 | 5.824 |
| NiSbTi | 6.177 | 6.169 | 6.167 | 6.160 |
| NiSnTi | 6.167 | 6.162 | 6.162 | 6.162 |
| NiSnZr | 6.467 | 6.459 | 6.462 | 6.467 |
| NiTiSn | 6.146 | 6.141 | 6.142 | 6.145 |
| PbYAu | 6.856 | 6.845 | 6.849 | 6.857 |
| PdHfSn | 6.483 | 6.477 | 6.474 | 6.481 |
| PdSbMn | 6.002 | 5.994 | 5.987 | 5.999 |
| PdTiGe | 5.980 | 5.971 | 5.973 | 5.972 |
| PdZrSn | 6.507 | 6.503 | 6.506 | 6.514 |
| PtHfSn | 6.449 | 6.442 | 6.439 | 6.448 |
| PtSbMn | 5.998 | 5.989 | 5.985 | 6.001 |
| PtSnMn | 5.996 | 5.990 | 5.990 | 6.007 |
| PtSnSc | 6.494 | 6.487 | 6.493 | 6.496 |
| PZnLi | 5.637 | 5.642 | 5.639 | 5.645 |
| RbZnBi | 7.694 | 7.683 | 7.689 | 7.697 |
| RhSbMn | 5.922 | 5.912 | 5.906 | 5.919 |
| RhTiGa | 5.917 | 5.907 | 5.910 | 5.910 |

TABLE VI: Continuation of tables IV and V.

| Element | $a_{\mathrm{AE}}$ | $a_{\mathrm{GBRV}}$ | $a_{\mathrm{VASP}}$ | $a_{\mathrm{PSLIB}}$ |
|---|---|---|---|---|
| SbCdAg | 6.688 | 6.693 | 6.693 | 6.679 |
| SbCdAu | 6.684 | 6.685 | 6.682 | 6.676 |
| SbCuCd | 6.566 | 6.570 | 6.567 | 6.554 |
| SbHgAg | 6.735 | 6.738 | 6.738 | 6.725 |
| SbScNi | 6.127 | 6.119 | 6.122 | 6.123 |
| SbScPd | 6.385 | 6.381 | 6.383 | 6.384 |
| SbScPt | 6.399 | 6.393 | 6.396 | 6.398 |
| SbTaCo | 5.983 | 5.971 | 5.970 | 5.970 |
| SbTaRu | 6.196 | 6.189 | 6.188 | – |
| SbTiCo | 5.896 | 5.897 | 5.894 | 5.902 |
| SbTiFe | 5.943 | 5.936 | 5.929 | 5.942 |
| SbTiNi | 5.965 | 5.956 | 5.953 | 5.957 |
| SbTiRu | 6.165 | 6.159 | 6.157 | – |
| SbVCo | 5.810 | 5.811 | 5.809 | 5.821 |
| SbVFe | 5.795 | 5.798 | 5.792 | 5.809 |
| SbVNi | 5.867 | 5.868 | 5.866 | 5.874 |
| SbVRu | 6.053 | 6.044 | 6.042 | – |
| SbYNi | 6.371 | 6.365 | 6.364 | 6.368 |
| SbYPt | 6.623 | 6.620 | 6.620 | 6.626 |
| SbZrRu | 6.347 | 6.343 | 6.342 | – |
| SbZrTc | 6.402 | 6.398 | 6.399 | 6.403 |
| ScSnAu | 6.518 | 6.512 | 6.515 | 6.521 |
| SnTiNi | 5.959 | 5.953 | 5.953 | 5.958 |
| SnTiPt | 6.239 | 6.231 | 6.236 | 6.239 |
| SrAlGa | 6.875 | 6.870 | 6.876 | 6.872 |
| SrCdSi | 6.966 | 6.966 | 6.974 | 6.961 |
| TlLiGe | 6.564 | 6.563 | 6.559 | 6.561 |
